# Supplementary material for: Stochastic Policy Gradient Ascent in Reproducing Kernel Hilbert Spaces
Source: arXiv:1807.11274 source file (2018-07-30)
Supplement: Supplementary file 1 [file appendix_bkp.tex]

%!TEX root = root.tex

%%%%%%%%%%%%%%%%%%%%%%%%%%%%%%%%%%%%%%%%%%%%%%%%%%%%%%%%%%%%%%%%%%%%%%%%%%%%%%%%%%%%%%%%%%%%%%%%%%%%%%%%%%%%%%%%%%%%%%%%%%%%%%%% S E C T I O N %%%%%%%%%%%%%%%%%%%%%%%%%%%%%%%%%%%%%%%%%%%%%%%%%%%%%%%%%%%%%%%%%%%%%%%%%%%%%%%%%%%%%%%%%%%%%%%%%%%%%%%%%%%%%%%%%%%%%%%%%%%%%%%%
%\section{Properties of the Discounted Reward}\label{sec_discounted_reward}
In this appendix we present some properties of the expected discounted reward and its gradient which are needed in the convergence analysis of functional stochastic gradient ascent. 
%
%%%%%%%%%%%%%%%%%%%%%%%%%%%%%%%%%%%%%%%%%%%%%%%%%%%%%%%%%%%%%%%%%%%%%%%%%%%%%%%%%%%%%%%%%%%%%%%%%%%%%%%%%%%%%%%%%%%  L E M M A %%%%%%%%%%%%%%%%%%%%%%%%%%%%%%%%%%%%%%%%%%%%%%%%%%%%%%%%%%%%%%%%%%%%%%%%%%%%%%%%%%%%%%%%%%%%%%%%%%%%%%%%%%%%%%%%%%%%%%%%%%%%%%%%%%%%%%%%%%%%%%
\begin{lemma}\label{lemma_bounded}
  Under Assumption \ref{assumption_reward_function} the expected discounted reward defined in \eqref{eqn_problem_statement} and the q-function defined in \eqref{eqn_q_function} satisfy
  \begin{equation}
    \left| U(h) \right| < \frac{B_r}{1-\gamma} \quad \mbox{and} \quad  
    \left| Q(s,a;h) \right| < \frac{B_r}{1-\gamma} \quad \forall \quad h\in\ccalH.
  \end{equation}
\end{lemma}
\begin{proof}
  The triangle inequality applied to $|U(h)|$, with $U(h)$ defined in \eqref{eqn_problem_statement}, yields  
  \begin{equation}
\left|U(h)\right| \leq \mathbb{E}\left[\left|\sum_{t=0}^\infty \gamma^tr(s_t,a_t)\right|\Big|h\right] \leq  \mathbb{E}\left[\sum_{t=0}^\infty \gamma^t|r(s_t,a_t)|\Big|h \right],
  \end{equation}
   Since the absolute value of the reward function $r(s,a)$ is bounded by $B_r$ for all $(s,a) \in \ccalS\times\ccalA$ (cf., Assumption \ref{assumption_reward_function}) it follows that
  \begin{equation}
\left|U(h)\right| \leq B_r \sum_{t=0}^\infty \gamma^t = \frac{B_r}{1-\gamma}.
  \end{equation}
  The proof of the result for $Q(s,a;h)$ is analogous. 
  \end{proof}
%
%%%%%%%%%%%%%%%%%%%%%%%%%%%%%%%%%%%%%%%%%%%%%%%%%%%%%%%%%%%%%%%%%%%%%%%%%%%%%%%%%%%%%%%%%%%%%%%%%%%%%%%%%%%%%%%%%%%  L E M M A %%%%%%%%%%%%%%%%%%%%%%%%%%%%%%%%%%%%%%%%%%%%%%%%%%%%%%%%%%%%%%%%%%%%%%%%%%%%%%%%%%%%%%%%%%%%%%%%%%%%%%%%%%%%%%%%%%%%%%%%%%%%%%%%%%%%%%%%%%%%%%

\begin{lemma}\label{lemma_bounded_gradient}
Let Assumption \ref{assumption_reward_function} hold, then $\nabla_h U(h,\cdot)$ defined as in \eqref{eqn_nabla_U} is bounded for all $h\in\ccalH$.
\end{lemma}
\begin{proof}
 Staring from  \eqref{eqn_nabla_U} and considering $\left\|k(s,\cdot)\right\| =1$ (cf., Definition \ref{def_rkhs}), one can write
\begin{equation}
  \left\|\nabla_h U(h,\cdot) \right\|\leq \frac{1}{1-\gamma}\mathbb{E}_{(s,a)\sim \rho(s,a)}\left[|Q(s,a;h)|\left\|\Sigma^{-1}\left(a-h(s)\right)\right\|\right].
\end{equation}
An then use the result of Lemma \ref{lemma_bounded} to further upper bound the norm of the gradient by 
\begin{equation}\label{eqn_norm_gradient_partial}
  \left\|\nabla_h U(h,\cdot) \right\|\leq \frac{B_r}{(1-\gamma)^2}\mathbb{E}_{(s,a)\sim \rho(s,a)}\left[\left\|\Sigma^{-1}\left(a-h(s)\right)\right\|\right].
\end{equation}
By construction $\Sigma^{-1/2}(a-h(s)$ is a multivariate normal distribution, hence the expectation of its norm is bounded. 
\end{proof}

%%%%%%%%%%%%%%%%%%%%%%%%%%%%%%%%%%%%%%%%%%%%%%%%%%%%%%%%%%%%%%%%%%%%%%%%%%%%%%%%%%%%%%%%%%%%%%%%%%%%%%%%%%%%%%%%%%%  L E M M A %%%%%%%%%%%%%%%%%%%%%%%%%%%%%%%%%%%%%%%%%%%%%%%%%%%%%%%%%%%%%%%%%%%%%%%%%%%%%%%%%%%%%%%%%%%%%%%%%%%%%%%%%%%%%%%%%%%%%%%%%%%%%%%%%%%%%%%%%%%%%%
\begin{lemma}\label{lemma_lipchitz}
  Let Assumption \ref{assumption_reward_function} hold. Then the gradient of the expected discounted reward satisfies 
  \begin{equation}
    \left\|\nabla_h U(h_1,\cdot) - \nabla_h U(h_2,\cdot)\right\|_\ccalH \leq L_1\|h_1-h_2\|_\ccalH+L_2\|h_1-h_2\|_{\ccalH}^2,
  \end{equation}
  for all $h_1,h_2 \in\ccalH$ with $L_1$ and $L_2$ given by 
  \begin{equation}\label{eqn_lipchitz_constants}
    L_1 = \frac{B_r}{\lambda_{\min}(\Sigma)(1-\gamma^2)}\left(\lambda_{\min}(\Sigma)+(\sigma_\pi^2-\sigma_\pi)+\frac{2\gamma\sigma_\pi}{(1-\gamma)}\right)   \quad \mbox{and}
  \end{equation}
  \begin{equation}
    L_2 = B_r\frac{2\gamma\sigma_\pi}{\lambda_{\min}(\Sigma)(1-\gamma)^3}.\nonumber
  \end{equation}
  where $B_r$ is the bound of the absolute value of the reward defined in Assumption \ref{assumption_reward_function} and $\sigma_\pi$ is the standard deviation of the Gaussian policy on each direction.
  \end{lemma}
\begin{proof}
  %
 % Let us start by considering the expression of $\nabla_h U(h,\cdot)$ given in \eqref{eqn_nabla_U} 
%\begin{equation}
%\nabla_h U(h,\cdot) = \frac{1}{1-\gamma}\mathbb{E}_{(s,a)\sim \rho(s,a)}\left[ Q(s,a;h)\kappa(s,\cdot)\Sigma^{-1}\left(a-h(s)\right) \Big| h\right].
%  \end{equation}
%
%In Proposition \ref{prop_unbiased_grad} we have showed that sampling from $\rho(s,a)$ is equivalent to drawing a geometric random variable $T$, and selecting $s$ and $a$ as the state action pair at time $T$. Hence, the previous expression can be written as 
%
%\begin{equation}
%\nabla_h U(h,\cdot) = \frac{1}{1-\gamma}\mathbb{E}\left[\sum_{t=0}^\infty \mathbbm{1}(T=t) Q(s_t,a_t;h)\kappa(s_t,\cdot)\Sigma^{-1}\left(a_t-h(s_t)\right) \Big| h\right].
%  \end{equation}
%
%In the proof of Proposition \eqref{prop_unbiased_grad} we argued that it was possible to exchange the sum and the expectation and that the draw of the random variable $T$ is independent of the evolution of the system (cf., \eqref{eqn_after_swaping_sum_expectation}). Hence we have that 
  %
  From the proof of Proposition \eqref{prop_unbiased_grad} (cf., \eqref{eqn_after_swaping_sum_expectation}) it holds
\begin{equation}
\begin{split}  
  \nabla_h U(h,\cdot) =\sum_{t=0}^\infty \gamma^t \mathbb{E}\left[ Q(s_t,a_t;h)\kappa(s_t,\cdot)\zeta^h_t \Big| h\right],
\end{split}
\end{equation}
where we have defined $\zeta^h_t:=\Sigma^{-1}\left(a_t-h(s_t)\right)$. Then, replacing the expression of $Q(s,a;h)$ by its definition in \eqref{eqn_q_function} the previous expression yields
  \begin{equation}
    \begin{split}
      \nabla_h U(h,\cdot) 
      & =\sum_{t=0}^\infty \gamma^{t}\mathbb{E}\left[\sum_{u=0}^\infty\gamma^u \mathbb{E}\left[r(s_{t+u},a_{t+u})|s_t,a_t\right]\kappa(s_t,\cdot)\zeta_t^h \right] \\
      &=\sum_{t=0}^\infty\sum_{u=0}^\infty \gamma^{t+u}\int r(s_{t+u},a_{t+u})\kappa(s_t,\cdot)\zeta^h_t\\
      &\quad \quad \quad \quad \quad p(s_0)\prod_{r=0}^{t+u}p(s_{r+1}|s_r,a_r) \pi_{h}(a_r|s_r)\,dsda \\
      &=\sum_{t=0}^\infty\sum_{u=0}^\infty \gamma^{t+u}\int r(s_{t+u},a_{t+u})\kappa(s_t,\cdot)\zeta^h_t \\
&\quad \quad \quad \quad \quad      P_{t+u}(s,a)\prod_{r=0}^{t+u} \pi_{h}(a_r|s_r)\,dsda,
\end{split}
    \end{equation}
where in the previous expression $P_{t+u}(s,a)$ is defined as 
  \begin{equation}
P_{t+u}(s,a) = p(s_0)\prod_{r=0}^{t+u} p(s_{r+1}|s_r,a_r),
  \end{equation}
  By defining the following function %
  \begin{equation}
  \Delta(h_1,h_2,s,a)=\zeta_t^{h_1}\prod_{r=0}^{t+u} \pi_{h_1}(a_r|s_r)-\zeta_t^{h_2}\prod_{r=0}^{t+u} \pi_{h_2}(a_r|s_r),
    \end{equation}
  one can write the difference $ \nabla_h U(h_1,\cdot) - \nabla_h U(h_2,\cdot)$ as 
  \begin{equation}
    \begin{split}
      \nabla_h U(h_1,\cdot) &- \nabla_h U(h_2,\cdot) =  \sum_{t=0}^\infty\sum_{u=0}^\infty \gamma^{t+u}\int r(s_{t+u},a_{t+u})\\
&      \kappa(s_t,\cdot)P_{t+u}(s,a)\Delta(h_1,h_2,s,a)\,dsda.
\end{split}
  \end{equation}
  Observe that by adding and subtracting $\zeta_t^{h_2}\prod_{r=0}^{t+u} \pi_{h_1}(a_r|s_r)$ to $\Delta(h_1,h_2,s,a)$ yields
   \begin{equation}\begin{split}
     \Delta(h_1,h_2,s,a)=\Sigma^{-1}(h_2(s_t)-h_1(s_t))\prod_{r=0}^{t+u} \pi_{h_1}(a_r|s_r)\\
     -\zeta_2^{h_2}\left(\prod_{r=0}^{t+u} \pi_{h_2}(a_r|s_r)-\prod_{r=0}^{t+u}\pi_{h_1}(a_r|s_r)\right).
\end{split}    \end{equation}
   and thus one can write $P_{t+u}(s+u)\Delta(h_1,h_2,s,a)$ as
   \begin{equation}\begin{split}
       P_{t+u}(s,a)\Delta(h_1,h_2,s,a) = \rho_{h_1}(s,a)\Sigma^{-1}\left(h_2(s_t)-h_1(s_t)\right) \\
       - P_{t+u}(s,a)\zeta_t^{h_2}\Delta_{\pi}(h_1,h_2,s,a), 
\end{split}     \end{equation}
   where we have defined 
   \begin{equation}
\Delta_{\pi}(h_1,h_2,s,a)  = \prod_{r=0}^{t+u}\pi_{h_2}(a_r|s_r)-\prod_{r=0}^{t+u}\pi_{h_1}(a_r|s_r).
     \end{equation}
   Then, the difference between the gradients is
     \begin{equation}
    \begin{split}
      \nabla_h U(h_1,\cdot) - \nabla_h U(h_2,\cdot) &=\sum_{t=0}^\infty\sum_{u=0}^\infty \gamma^{t+u}\int r(s_{t+u},a_{t+u})\kappa(s_t,\cdot)
      \\
      &\quad \quad \Sigma^{-1} \rho_{h_1}(s,a)\left(h_2(s_t)-h_1(s_t)\right)\,dsda\\
      &-\sum_{t=0}^\infty\sum_{u=0}^\infty \gamma^{t+u}\int r(s_{t+u},a_{t+u})\kappa(s_t,\cdot)\zeta_t^{h_2} \\
      & \quad\quad P_{t+u}(s,a)\Delta_{\pi}(h_1,h_2,s,a)\,dsda\\
\end{split}
  \end{equation}
Using the triangle inequality, the norm of the difference can be upper bounded by 
     \begin{equation}\label{eqn_upper_bound_norms1}
    \begin{split}
      \left\|\nabla_h U(h_1,\cdot) - \nabla_h U(h_2,\cdot)\right\| &\leq\sum_{t=0}^\infty\sum_{u=0}^\infty \gamma^{t+u}B_r\left\|\Sigma^{-1}\right\| \\
      &\int \rho_{h_1}(s,a)\left\|h_2(s_t)-h_1(s_t)\right\|\,dsda\\
      &+\sum_{t=0}^\infty\sum_{u=0}^\infty \gamma^{t+u}B_r \\
      &\int  P_{t+u}(s,a)\zeta_t^{h_2}\left|\Delta_{\pi}(h_1,h_2,s,a)\right|\,dsda. 
\end{split}
  \end{equation}
The integral in the first term is upper bounded by virtue of the Cauchy-Schwartz inequality as 
     \begin{equation}
       \begin{split}
         \int \rho_{h_1}(s,a)\left\|h_2(s_t)-h_1(s_t)\right\|\,dsda \leq \\
         \int \rho_{h_1}(s,a)\left|\left\langle h_2-h_1,\kappa(s_t,\cdot)\right \rangle_\ccalH\right|\,dsda \leq \\
     \int \rho_{h_1}(s,a)\left\|h_2-h_1\right\|\,dsda  =\left\|h_2-h_1\right\|.
         \end{split}
     \end{equation}
     Therefore the first term in on the right hand side of \eqref{eqn_upper_bound_norms1} is upper bounded by
     \begin{equation}
       \begin{split}
         \sum_{t=0}^\infty\sum_{u=0}^\infty \gamma^{t+u}B_r\left\|\Sigma^{-1}\right\| \left\|h_1-h_2\right\|\leq         \frac{B_r}{(1-\gamma)^2\lambda_{\min}\left(\Sigma\right)} \left\|h_1-h_2\right\|.
         \end{split}
\end{equation}
     We next work towards bounding the second term in \eqref{eqn_upper_bound_norms1}. In particular we focus on the term $\Delta_{\pi}(h_1,h_2,s,a)$. Let $h_{\lambda} = \lambda h_1+(1-\lambda)h_2$ with $\lambda\in [0,1]$ and write
     \begin{equation} \begin{split}
\Delta_{\pi}(h_1,h_2,s,a) =\sum_{r=0}^{t+u} \left\langle z_r^{h_\lambda}\prod_{r=0}^{t+u}\pi_{h_\lambda}(a_r|s_r) ,h_1-h_2\right\rangle
         \end{split} \end{equation}
%     \begin{equation}\begin{split}
%       \Delta_{\pi}(h_1,h_2,s,a) = \frac{1}{\sqrt{det\left(2\pi \Sigma_{\pi}\right)}}\Sigma_{\pi}^{-1} \\
%\left\langle\sum_{r=0}^{t+u}(a_r-h_{\lambda}(s_r))e^{-\sum_{r=0}^{t+u}(a_r-h_\lambda(s_r))^\top \Sigma_{\pi}^{-1}(a_r-h_\lambda(s_r))}\kappa(s_r,\cdot),h_1-h_2 \right\rangle
%\end{split}     \end{equation}
     %
     Thus the absolute value of the previous difference can be upper bounded using the Cauchy-Schwartz inequality by
     \begin{equation}
\left|\Delta_{\pi}(h_1,h_2,s,a) \right|        \leq \left\|h_1-h_2\right\|\sum_{r=0}^{t+u}\left|\zeta_r^{h_\lambda}\right|\prod_{r=0}^{t+u} \pi_{h_\lambda}(a_r|s_r).
       \end{equation}
     The integral of the second term in \eqref{eqn_upper_bound_norms1} is therefore upper bounded by

     \begin{equation}
       \begin{split}
                &\int  P_{t+u}(s,a)\left|\zeta_t^{h_2}\right|\left|\Delta_{\pi}(h_1,h_2,s,a)\right|\,dsda
       \leq \\
       &\leq \left\|h_1-h_2\right\|\int  P_{t+u}(s,a)\left|\zeta_t^{h_2}\right|\sum_{r=0}^{t+u}\left|\zeta_r^{h_\lambda}\right| \prod_{r=0}^{t+u} \pi_{h_\lambda}(a_r|s_r)\,dsda \\
       &\leq \left\|h_1-h_2\right\|\int  P_{t+u}(s,a)\left|\zeta_t^{h_\lambda}\right|\sum_{r=0}^{t+u}\left|\zeta_r^{h_\lambda}\right| \prod_{r=0}^{t+u} \pi_{h_\lambda}(a_r|s_r)\,dsda \\
       &+ \left\|h_1-h_2\right\|^2\int  P_{t+u}(s,a)\sum_{r=0}^{t+u}\left|\zeta_r^{h_\lambda}\right| \prod_{r=0}^{t+u} \pi_{h_\lambda}(a_r|s_r)\,dsda \\
       & \leq \sigma_\pi(t+u)\left(\left\|h_1-h_2\right\|+\left\|h_1-h_2\right\|^2\right) \\
       &+ \left\|h_1-h_2\right\|(\sigma_\pi^2-\sigma_\pi)\\
\end{split}
     \end{equation}
     Thus, the norm of the difference of gradients in \eqref{eqn_upper_bound_norms1} is upper bounded by
     \begin{equation}
       \begin{split}
         \left\|\nabla_h U(h_1,\cdot)-\nabla_h U(h_2,\cdot) \right\| \leq \frac{B_r}{\lambda_{\min}\left(\Sigma\right)(1-\gamma)^2}\left\| h_1-h_2\right\|\\
         +       \frac{B_r}{(1-\gamma)^2}\left\|h_1-h_2 \right\|\left(\sigma_\pi^2-\sigma_\pi\right) \\
         +B_r\sigma_\pi\left(\left\|h_1-h_2\right\|^2+\left\|h_1-h_2 \right\|\right)\sum_{t=0}^\infty\sum_{u=0}^\infty (t+u)\gamma^{t+u}.
         \end{split}
       \end{equation}
     The double sum yields
     \begin{equation}
\sum_{t=0}^\infty\sum_{u=0}^\infty (t+u)\gamma^{t+u} = \frac{2\gamma}{(1-\gamma)^3},
     \end{equation}
     which completes the proof with $L_1$ and $L_2$ defined as in \eqref{eqn_lipchitz_constants}.
  \end{proof}
%%%%%%%%%%%%%%%%%%%%%%%%%%%%%%%%%%%%%%%%%%%%%%%%%%%%%%%%%%%%%%%%%%%%%%%%%%%%%%%%%%%%%%%%%%%%%%%%%%%%%%%%%%%%%%%%%%%%%%%%%%%%%%%% S E C T I O N %%%%%%%%%%%%%%%%%%%%%%%%%%%%%%%%%%%%%%%%%%%%%%%%%%%%%%%%%%%%%%%%%%%%%%%%%%%%%%%%%%%%%%%%%%%%%%%%%%%%%%%%%%%%%%%%%%%%%%%%%%%%%%%%
%\section{Properties of the stochastic gradient}\label{app_stochastic_gradient}
%
%%%%%%%%%%%%%%%%%%%%%%%%%%%%%%%%%%%%%%%%%%%%%%%%%%%%%%%%%%%%%%%%%%%%%%%%%%%%%%%%%%%%%%%%%%%%%%%%%%%%%%%%%% P R O P O S I T I O N %%%%%%%%%%%%%%%%%%%%%%%%%%%%%%%%%%%%%%%%%%%%%%%%%%%%%%%%%%%%%%%%%%%%%%%%%%%%%%%%%%%%%%%%%%%%%%%%%%%%%%%%%%%%%%%%
\begin{lemma}\label{lemma_stochastic_gradient}
  The second and third moments of the estimate $\hat{\nabla}_h U(h,\cdot)$ are bounded by
  \begin{equation}\label{eqn_moment_bounds}
\mathbb{E}\left[\left\|\hat{\nabla}_h U(h,\cdot) \right\|^2\right] \leq \sigma^2 \quad \mbox{and} \quad \mathbb{E}\left[\left\|\hat{\nabla}_h U(h,\cdot) \right\|^3\right] \leq \sigma^{3}, 
  \end{equation}
  with 
  \begin{equation}
    %  \sigma = \frac{B_r}{(1-\gamma)}\left(2\sum_{k=0}^\infty k^6(1-\gamma)\gamma^k8\frac{\Gamma(3+p/2)}{\Gamma(p/2)}\right)^{1/6},
      \sigma= \frac{(3\gamma)^{1/3}}{(1-\gamma)^2}\frac{1}{\lambda_{\min}\left(\Sigma^{1/2}\right)}\left(4\frac{\Gamma(2+p/2)}{\Gamma(p/2)}\right)^{1/4}.
  \end{equation}
  where $\Gamma(\cdot)$ is the Gamma function.
\end{lemma}
\begin{proof}
Let us start by bounding the cube the norm of the stochastic gradient defined in \eqref{eqn_stochastic_grad}.
\begin{align}
\nonumber  \left\|  \hat{\nabla}_hU(h,\cdot)\right\|^3 &\leq \frac{1}{8(1-\gamma)^3}\left\|\hat{Q}(s_T,a_T;h)-\hat{Q}(s_T,\bar{a}_T;h)\right\|^3 \\
  &\times\left\|\kappa(s_T,\cdot)\right\|^3\left\|\Sigma^{-1}(a_T-h(s_T))\right\|^3.
\label{eq_bound_nablau}\end{align}
Using the fact that $\left\| \kappa(s_t,\cdot)\right\| = 1$ (cf., Definition \ref{def_rkhs}) and the fact that the difference between estimates of Q is bounded by $B_r (T_{Q}+T_Q^\prime)$, \eqref{eq_bound_nablau} is upper bounded by 
\begin{equation}\nonumber
\left\|  \hat{\nabla}_hU(h,\cdot)\right\|^3 \leq\frac{B_r^3}{8(1-\gamma)^3}(T_Q+T_Q^\prime)^3 \left\|\Sigma^{-1}(a_T-h(s_T))\right\|^3.
\end{equation}
From the independence of $T_Q$ and $T_Q^\prime$ with respect to the state evolution, and the monotonicity of the expectation, it results 
\begin{equation}\label{eqn_product_expectations}
  \begin{split}
  \mathbb{E}\left[\left\|  \hat{\nabla}_hU(h,\cdot)\right\|^3\right] \leq \frac{B_r^3}{8(1-\gamma)^3}\mathbb{E}\left[\left(T_Q+T_Q^\prime\right)^3\right]\\
    \times \mathbb{E}\left[\left\|\Sigma^{-1}(a_T-h(s_T))\right\|^3\right].
  \end{split}
\end{equation}
The sum of two independent geometric variables satisfies
\begin{equation}
\nonumber P(T_Q+T_Q^\prime=k) = (1-\gamma)^2(k+1) \gamma^k.
\end{equation} 
%
%Since the two random variables are independent the previous expression reduces to 
%
%\begin{equation}\begin{split}
 %   P(\max(T_Q,T_Q^\prime)=k) =  (1-\gamma)\gamma^k (1-\gamma^{k+1}) \\
  %  + (1-\gamma)\gamma^k(1-\gamma^k) = (1-\gamma)\gamma^k(2-\gamma^k-\gamma^{k+1}).
%\end{split}\end{equation} 
%
Thus, the third moment is upper bounded by
\begin{align}
    \nonumber \mathbb{E}\left[(T_Q+T_Q^\prime)^3\right] &= \sum_{k=0}^\infty k^3 (1-\gamma)^2(k+1)\gamma^k\\
		&= \frac{\gamma(1+14\gamma+8\gamma^2)}{(1-\gamma)^3}\leq \frac{23 \gamma}{(1-\gamma)^3}   \label{exp_sum_geom}   \end{align} 
where the last inequality follows from the fact that $\gamma<1$. On the other hand observe that $\left\|\Sigma^{-1/2}a_T-h(s_T)\right\|^2$ is Chi-squared with parameter $p$ since it is a sum of squares of normal random variables. Hence, the second expectation in \eqref{eqn_product_expectations} can be bounded using Jensen's inequality by, 
\begin{align}
   \nonumber &\mathbb{E}\left[\left\|\Sigma^{-1}(a_T-h(s_T))\right\|^3\right] \leq \frac{1}{\lambda_{\min}(\Sigma^{1/2})^{3}}\mathbb{E}\left[\chi_p^{3/2}\right]\\
    %\leq \frac{1}{\lambda_{\min}(\Sigma^{1/2})^{3}}\left(8\frac{\Gamma(3+p/2)}{\Gamma(p/2)}\right)^{3/2}.
     &\leq \frac{1}{\lambda_{\min}(\Sigma^{1/2})^{3}}\mathbb{E}\left[\chi_p^{2}\right]^{3/4} =\frac{1}{\lambda_{\min}(\Sigma^{1/2})^{3}}\left(4\frac{\Gamma(2+p/2)}{\Gamma(p/2)}\right)^{3/4}\label{bound_gaussian_cube}
  \end{align}
Substituting \eqref{exp_sum_geom} and \eqref{bound_gaussian_cube} in \eqref{eqn_product_expectations} yields the the bound for the  third moment of the stochastic gradient  in  \eqref{eqn_moment_bounds}. To validate the bound on the second moment consider $x=\left\|  \hat{\nabla}_hU(h,\cdot)\right\|^3$ and observe that since $x^{2/3}$ is a concave function one can reverse Jensen's inequality  to obtain %   = \left(\left\|  \hat{\nabla}_hU(h,\cdot)\right\|^2\right)^{3/2}$. Since  is a convex function, Jensen's inequality implies that   
\begin{equation}\nonumber
\mathbb{E}\left[\left(\left\|  \hat{\nabla}_hU(h,\cdot)\right\|^3\right)^{2/3}\right]\leq  \mathbb{E}\left[\left\|  \hat{\nabla}_hU(h,\cdot)\right\|^3\right]^{2/3} \leq \left(\sigma^3\right)^{2/3}   
  \end{equation}
  which completes the proof. \end{proof}

%%%%%%%%%%%%%%%%%%%%%%%%%%%%%%%%%%%%%%%%%%%%%%%%%%%%%%%%%%%%%%%%%%%%%%%%%%%%%%%%%%%%%%%%%%%%%%%%%%%%%%%%%% P R O P O S I T I O N %%%%%%%%%%%%%%%%%%%%%%%%%%%%%%%%%%%%%%%%%%%%%%%%%%%%%%%%%%%%%%%%%%%%%%%%%%%%%%%%%%%%%%%%%%%%%%%%%%%%%%%%%%%%%%%%
\begin{lemma}\label{lemma_square_int_martingale}
Let $e_j=\hat{\nabla}_h U(h_j)-{\nabla}_h U(h_j)$ and let $\eta_j$ be such that it satisfies \eqref{eqn_stepsize}. Then, the sequence  
  \begin{equation}\label{eqn_martingale_appendix}
S_k  =\sum_{j=0}^k \eta_j e_j,
      \end{equation}
  converges to a finite limit with probability one.
\end{lemma}
\begin{proof}
  By virtue of Theorem 5.4.9 \cite{durrett2010probability}), it suffices to show that $S_k$ is a square integrable margingale and that
  \begin{equation}\label{eqn_last_condition_square_integrable}
\lim_{n\to\infty} \sum_{m=1}^n \mathbb{E}\left[(S_m-S_{m-1})^2\big| \ccalF_{m}\right] <\infty \quad \mbox{a.e.}
  \end{equation}

Recall that the estimate of the gradient is unbiased, i.e. $\mathbb{E}\left[ \hat{\nabla}_h U(h_k,\cdot)\big|\ccalF_k\right]={\nabla}_h U(h_k,\cdot)$, hence we have that $\mathbb{E}\left[ e_k\big|\ccalF_k\right]=0$. This allows us to write 
            \begin{equation}
\mathbb{E}\left[S_k\big|\ccalF_k\right] = S_{k-1} + \mathbb{E}\left[\eta_ke_k\big|\ccalF_k\right] = S_{k-1}.
              \end{equation}
            Thus $S_k$ is a martingale. To show that it is square integrable, observe that we can compute squared norm of $S_k$ as
            \begin{equation}\begin{split}
              \left\|S_k\right\|^2 = \left\|\sum_{j=0}^k \eta_je_j\right\|^2 = \eta_k^2\|e_k\|^2+2\eta_ke_k^\top\sum_{j=0}^{k-1}\eta_je_j \\+ \left\|\sum_{j=0}^{k-1} \eta_je_j\right\|^2 
              = \eta_k^2\|e_k\|^2 + 2\eta_k e_k^\top S_{k-1} + \left\|S_{k-1}\right\|^2.
              \end{split}\end{equation}
            Take the expectation with respect to the sigma field $\ccalF_k$ and use the fact that $\mathbb{E}\left[ e_k\big|\ccalF_k\right]=0$ to write
            \begin{equation}
              \mathbb{E}\left[\left\|S_k\right\|^2\big|\ccalF_k\right] = \eta_k^2\mathbb{E}\left[\|e_k\|^2\big|\ccalF_k\right]+\left\|S_{k-1}\right\|^2.
            \end{equation}
            The previous expression implies that
                        \begin{equation}
              \mathbb{E}\left[\left\|S_k\right\|^2\right] = \eta_k^2\mathbb{E}\left[\|e_k\|^2\right]+\mathbb{E}\left[\left\|S_{k-1}\right\|^2\right].
                        \end{equation}
           Recursively we have that
                        \begin{equation}
                          \mathbb{E}\left[\left\|S_k\right\|^2\right] = \sum_{j=0}^k\eta_j^2\mathbb{E}\left[\|e_j\|^2\right].
                          \end{equation}
                        Since the step sizes are square summable and the second moment of the error is bounded (cf., lemmas \ref{lemma_bounded_gradient} and \ref{lemma_stochastic_gradient}) the second moment of $S_k$ is bounded for all $k$. We next show that \eqref{eqn_last_condition_square_integrable} holds. Observe that by definition of $S_k$ (cf., \eqref{eqn_martingale_appendix}) one can write 
                        \begin{equation}\begin{split}
\sum_{m=1}^n \mathbb{E}\left[\|S_m-S_{m-1}\|^2\big|\ccalF_{m}\right]=\sum_{m=1}^n \mathbb{E}\left[\|\eta_me_m\|^2\big|\ccalF_{m}\right] \\= \sum_{m=1}^n \eta_m^2 \mathbb{E}\left[\|e_j\|^2\big|\ccalF_m\right].
\end{split}                          \end{equation}
                        Which is bounded for all $n$ as it was previously argued. This completes the proof that $\lim_{k\to\infty} S_k$ converges to a finite random variable with probability one.

\end{proof}
